# Supplementary material for: Remote Attestation: A Literature Review
Source: arXiv:2105.02466 source file (2021-05-12)
Supplement: Supplementary file 1 [file Appendix.tex]

\appendix

\section{RA Principles}
\label{apx:principles}
\subsection{Principles of Remote Attestation~\cite{principles_of_remote_attestation}}
\begin{description}
    \item[Fresh information] Assertions about the prover should reflect the running system, rather than just disk images.
    \item[Comprehensive information] Attestation mechanisms should be capable of delivering comprehensive information about the prover.
    \item[Constrained disclosure] A prover should be able to enforce policies governing which measurements are sent to each verifier.
    \item[Semantic explicitness] The semantic content of attestations should be explicitly presented in logical form and be composable using valid logical inferences.
    \item[Trustworthy mechanism] Verifiers should receive evidence of the trustworthiness of the attestation mechanisms on which they rely. In particular, the attestation architecture in use should be identified to both verifier and prover.
\end{description}

\subsection{A Minimalist Approach to Remote Attestation~\cite{minimalist}:}
\begin{description}
    \item[Exclusive access] Based on the Att-Forge security game, a prover's attestation mechanism should have exclusive access to the secret k. 
    \item[No leaks] The attestation mechanism should not leak any function of the secret k.
    \item[Immutability] The code of the attestation mechanism is immutable. Otherwise we risk a Time-Of-Check-To-Time-Of-Use (TOCTTOU) attack, which can be prevented by a hardware signature check of the code.
    \item[Uninterruptability] Execution of the attestation mechanism must be uninterruptible.
    \item[Controlled invocation] The attestation mechanism must only be invoked from its intended entry point.
\end{description}
